# Supplementary material for: Probing the theoretical description of central exclusive production
Source: arXiv:1006.4494 source file (2010-06-23)
Supplement: Supplementary file 1 [file Appendix.tex]

\section{Large top mass effective theory}\label{app:largetop}
%%%%%%%%%%%%%%%%%%%%%%%%%%

In this appendix we describe the effective theory, formed by taking the top quark mass to infinity~\cite{Shifman:1979eb,Voloshin:1985tc,Ellis:1975ap} which we use to compute the next-to-leading order corrections to central exclusive Higgs production. This approach has been found to give good agreement with the full theory, provided that the Higgs mass satisfies $m_H \lesssim 2 m_{\textrm{top}}$ and the transverse momenta of any jets produced in association with the Higgs satisfy $p_\perp \lesssim m_{\textrm{top}}$~\cite{DelDuca:2001fn,DelDuca:2003ba}.

We work in a theory in which the top quark has been integrated out and all other quarks are taken as massless. In this approach, the only coupling of the Higgs is to gluons\footnote{We consistently ignore electroweak couplings throughout.}, via the following term in the effective Lagrangian 
\begin{equation} \label{eq:LeffBare}
  \mathcal{L}_{\text{eff}}=-\frac{H}{4}C^0_1\mathcal{O}^0_1\;, \qquad \mathcal{O}^0_1=(G_0)^a_{\mu\nu}(G_0)^{a \mu\nu}
\end{equation}
where $C^0_1$ is a coefficient function, zeroes indicate that these are bare quantities and it is understood that they are defined in the five flavour effective theory. Both $C^0_1$ and matrix elements of $\mathcal{O}^0_1$ contain ultraviolet divergences, however their product is finite,
%(I have seen this stated and there must be some simple way of seeing this is the case, but at the moment it is eluding me!).
since the operator in the full theory which (\ref{eq:LeffBare}) approximates ($\frac{H}{v}m_t\bar{\psi}\psi$) is a conserved current. 

Using the Bogolyubov-Parasiuk R-operation~\cite{Bogolyubov:1980nc,Spiridonov:1984br}, it is possible to define a finite version of $\mathcal{O}^0_1$, which we denote $\mathcal{O}^R_1$. This finite operator may then be related to the bare operator as~\cite{Spiridonov:1984br}
\begin{equation}
	\mathcal{O}^R_1 = Z_{\mathcal{O}_1} \mathcal{O}^0_1\;, \qquad
	Z_{\mathcal{O}_1} =  \frac{1}{1-\beta(\mathcal{N}\alpha_s)/\epsilon}
\end{equation}
where 
\begin{equation}
	\mathcal{N} = \text{exp}[\epsilon(-\gamma_{\text{E}} + \ln(4\pi))],
\end{equation}
and $\beta(\alpha_s)$ and $\alpha_s \equiv \alpha_s(\mu)$ are the QCD beta function and the $\overline{\textrm{MS}}$ running coupling respectively. Again, both are defined in the five flavour theory.

The effective Lagrangian now reads

\begin{equation}
	\mathcal{L}_{\text{eff}}=-\frac{H}{4}C^R_1\mathcal{O}^R_1\; \qquad C^R_1 = Z_{\mathcal{O}_1}^{-1} C^0_1 \label{eq:RewrittenLeff}\;.
\end{equation}
Since both matrix elements of $\mathcal{O}^R_1$ and the full expression are finite, $C^R_1$ is also finite and is given by
\begin{equation}
	C^R_1(\mu) = -\frac{1}{3v}\frac{\alpha_s(\mu)}{\pi}\left( 1 + \frac{11}{4}\frac{\alpha_s(\mu)}{\pi}   \right) + \mathcal{O}(\alpha_s^3)
\end{equation}
where again $\alpha_s(\mu)$ is the five flavour $\overline{\textrm{MS}}$ running coupling and $v$ is the Higgs vacuum expectation value.

%%%%%%%%%%%%%%%%%%%%%%%%%%%%%%%%%%%%%%%%%
\begin{figure}[t]
	 \subfigure{\includegraphics[width=0.8\textwidth]{FeynmanDiagrams/LargeTopFeynman/1/1.epsi} }\\
	 \subfigure{\includegraphics[width=0.7\textwidth]{FeynmanDiagrams/LargeTopFeynman/2/2.epsi}}\\
	\subfigure{\includegraphics[width=0.7\textwidth]{FeynmanDiagrams/LargeTopFeynman/3/3.epsi}}
	\caption{Feynman rules for the large top mass effective theory. See the text for the definitions of $V_3$ and $V_4$.}\label{fig:LargeTopFeynman}
\end{figure}
%%%%%%%%%%%%%%%%%%%%%%%%%%%%%%%%%%%%%%%%%

The Feynman rules generated by equation~(\ref{eq:RewrittenLeff}) are displayed in figure~\ref{fig:LargeTopFeynman}, and can be written in terms of the standard three and four gluon vertices:
\begin{align}
	V_{3,\mu_1\mu_2\mu_3}^{a_1a_2a_3}(k_1,k_2,k_3) &= g f^{a_1a_2a_3}\big( g_{\mu_1\mu_2}(k_1-k_2)_{\mu_3} + g_{\mu_2\mu_3}(k_2-k_3)_{\mu_1} \nonumber \\
	& \qquad \qquad \qquad + g_{\mu_3\mu_1}(k_3-k_1)_{\mu_2} \big) \\
	V_{4,\mu_1\mu_2\mu_3\mu_4}^{a_1a_2a_3a_4}(k_1,k_2,k_3,k_4) &= -i g^2 \big( f^{a_1a_2e}f^{a_4a_3e}( g_{\mu_1\mu_4}g_{\mu_2\mu_3} - g_{\mu_1\mu_3}g_{\mu_4\mu_2}  ) \nonumber \\
	&  \qquad \qquad  f^{a_1a_3e}f^{a_4a_2e}( g_{\mu_1\mu_4}g_{\mu_2\mu_3} - g_{\mu_1\mu_2}g_{\mu_4\mu_3}  ) \nonumber \\
	&  \qquad \qquad  f^{a_1a_4e}f^{a_2a_3e}( g_{\mu_1\mu_2}g_{\mu_4\mu_3} - g_{\mu_1\mu_3}g_{\mu_4\mu_2}  )  \big) \;.
\end{align}
